# Supplementary material for: Causal Models for Growing Networks
Source: arXiv:2504.01012 source file (2025-04-01)
Supplement: Supplementary file 1 [file 006Appendix1_HowRelationsRelate.tex]

\section{How Relations Relate}
\label{appendix:enumeration}
\spacebefsection

With respect to the total ordering of the nodes, there are $13$ ways in which two dyads can relate:
% \vspace{-20pt}
\begin{align*}
    \BoxNodeOne{} \BoxNodeTwo{} \UnBoxNode{i} \UnBoxNode{} \UnBoxNode{} \UnBoxNode{j} \UnBoxNode{} \UnBoxNode{}\\
    \BoxNodeOne{} \UnBoxNode{} \BoxNodeTwo{i} \UnBoxNode{} \UnBoxNode{} \UnBoxNode{j} \UnBoxNode{} \UnBoxNode{}\\
    \BoxNodeOne{} \UnBoxNode{} \UnBoxNode{i} \BoxNodeTwo{} \UnBoxNode{} \UnBoxNode{j} \UnBoxNode{} \UnBoxNode{}\\
    \BoxNodeOne{} \UnBoxNode{} \UnBoxNode{i} \UnBoxNode{} \UnBoxNode{} \BoxNodeTwo{j} \UnBoxNode{} \UnBoxNode{}\\
    \BoxNodeOne{} \UnBoxNode{} \UnBoxNode{i} \UnBoxNode{} \UnBoxNode{} \UnBoxNode{j} \BoxNodeTwo{} \UnBoxNode{}\\
    \UnBoxNode{} \UnBoxNode{} \BoxNodeOne{i} \BoxNodeTwo{} \UnBoxNode{} \UnBoxNode{j} \UnBoxNode{} \UnBoxNode{}\\
    \UnBoxNode{} \UnBoxNode{} \BoxNodeOne{i} \UnBoxNode{} \UnBoxNode{} \BoxNodeTwo{j} \UnBoxNode{} \UnBoxNode{}\\
    \UnBoxNode{} \UnBoxNode{} \BoxNodeOne{i} \UnBoxNode{} \UnBoxNode{} \UnBoxNode{j} \BoxNodeTwo{} \UnBoxNode{}\\
    \UnBoxNode{} \UnBoxNode{} \UnBoxNode{i} \BoxNodeOne{} \BoxNodeTwo{} \UnBoxNode{j} \UnBoxNode{} \UnBoxNode{}\\
    \UnBoxNode{} \UnBoxNode{} \UnBoxNode{i} \BoxNodeOne{} \UnBoxNode{} \BoxNodeTwo{j} \UnBoxNode{} \UnBoxNode{}\\
    \UnBoxNode{} \UnBoxNode{} \UnBoxNode{i} \BoxNodeOne{} \UnBoxNode{} \UnBoxNode{j} \BoxNodeTwo{} \UnBoxNode{}\\
    \UnBoxNode{} \UnBoxNode{} \UnBoxNode{i} \UnBoxNode{} \UnBoxNode{} \BoxNodeOne{j} \BoxNodeTwo{} \UnBoxNode{}\\
    \UnBoxNode{} \UnBoxNode{} \UnBoxNode{i} \UnBoxNode{} \UnBoxNode{} \UnBoxNode{j} \BoxNodeOne{} \BoxNodeTwo{}
\end{align*}
% \vspace{-10pt}
However, we would like our meta-DAGs to have finite ancestral sets, so it is easy to sample from them. 
% *** maybe comment of how 
This excludes the five options with circles appearing after $j$, 
as they represent causal arrows from infinitely many dyads with indices greater than $j$,
leaving the options displayed in {\refTypeCausalArrows}, which we study throughout the paper. 
