# Supplementary material for: Causal Models for Growing Networks
Source: arXiv:2504.01012 source file (2025-04-01)
Supplement: Supplementary file 2 [file 006Appendix3_HasseDiagramOLD.tex]

% \newpage
\section{Hasse Diagram with the 21 Invariant Causal Models}
\label{appendixFigHasse}
\begin{figure}
\begin{center}
\begin{tikzpicture}[scale=1, every node/.style={circle,draw,align=center}]
    \tikzmath{\HasseSpacingH=3.0;\HasseSpacingV=2.95;}
    \newcommand{\NodeScale}{1.4cm}
    \tikzmath{\ZeroScale=0.71;\OneScale=1.0;\TwoScale=1.41;\ThreeScale=1.73;\FourScale=2.0;
    \FiveScale=2.236;\SixScale=2.5;\SevenScale=1.0;}
    \newcommand{\OneSize}{1cm}
    \newcommand{\TwoSize}{1.41cm}
    \newcommand{\ThreeSize}{1.73cm}
    \newcommand{\FourSize}{2cm}
    \newcommand{\FiveSize}{2.236cm}
    \newcommand{\SixSize}{2.45cm}
    \newcommand{\SevenSize}{0.71cm}
     \newcommand{\innersep}{0.015cm}
    % Nodes
    \node[minimum size=\NodeScale*\ZeroScale, inner sep=\innersep] (empty) at (0,0) {};%$\emptyset$
    
    \node[minimum size=\NodeScale*\OneScale, inner sep=\innersep] (dj) at (-2*\HasseSpacingH,\HasseSpacingV) {\OldName};
    \node[minimum size=\NodeScale*\OneScale, inner sep=\innersep] (dd) at (-\HasseSpacingH,\HasseSpacingV) {\FarName};
    \node[minimum size=\NodeScale*\OneScale, inner sep=\innersep] (ir) at (0,\HasseSpacingV) {\HubName};
    \node[minimum size=\NodeScale*\OneScale, inner sep=\innersep] (rr) at (\HasseSpacingH,\HasseSpacingV) {\NearName};
    \node[minimum size=\NodeScale*\OneScale, inner sep=\innersep] (rj) at (2*\HasseSpacingH,\HasseSpacingV) {\NewName};
    
    \node[minimum size=\NodeScale*\TwoScale, inner sep=\innersep] (djdd) at (-2*\HasseSpacingH,2*\HasseSpacingV) {\OldName/\FarName}; 
    \node[minimum size=\NodeScale*\TwoScale, inner sep=\innersep] (di) at (-1*\HasseSpacingH,2*\HasseSpacingV) {\PathName \\ (\FarName)};
    \node[minimum size=\NodeScale*\TwoScale, inner sep=\innersep] (ddir) at (0*\HasseSpacingH,2*\HasseSpacingV) {\FarName/\HubName}; 
    \node[minimum size=\NodeScale*\TwoScale, inner sep=\innersep] (irrr) at (1*\HasseSpacingH,2*\HasseSpacingV) {\HubName/\NearName}; 
    \node[minimum size=\NodeScale*\TwoScale, inner sep=\innersep] (rrrj) at (2*\HasseSpacingH,2*\HasseSpacingV) {\NearName/\NewName}; 

    \node[minimum size=\NodeScale*\ThreeScale, inner sep=\innersep] (djdi) at (-2*\HasseSpacingH,3*\HasseSpacingV) {\OldName/\PathName\\ (\FarName)}; 
    \node[minimum size=\NodeScale*\ThreeScale, inner sep=\innersep] (dr) at (-1*\HasseSpacingH,3*\HasseSpacingV) {\MidName \\ (\PathName/\FarName)};
    \node[minimum size=\NodeScale*\ThreeScale, inner sep=\innersep] (diir) at (0*\HasseSpacingH,3*\HasseSpacingV) {\PathName/\HubName \\ (\FarName)};
    \node[minimum size=\NodeScale*\ThreeScale, inner sep=\innersep] (irrj) at (2*\HasseSpacingH,3*\HasseSpacingV) {\HubName/\NewName \\ (\NearName)};
    
    \node[minimum size=\NodeScale*\FourScale, inner sep=\innersep] (djdr) at (-2*\HasseSpacingH,4*\HasseSpacingV) {\OldName/\MidName \\ (\PathName/\FarName)};
    \node[minimum size=\NodeScale*\FourScale, inner sep=\innersep] (drir) at (0*\HasseSpacingH,4*\HasseSpacingV) {\MidName/\HubName \\ (\PathName/\FarName)};

    \node[minimum size=\NodeScale*\FiveScale, inner sep=\innersep] (djir) at (-1*\HasseSpacingH,5*\HasseSpacingV) {\OldName/\HubName \\ (\MidName\PathName/\FarName)}; 
    \node[minimum size=\NodeScale*\FiveScale, inner sep=\innersep] (drrr) at (1*\HasseSpacingH,5*\HasseSpacingV) {\MidName/\NearName \\ (\PathName/\FarName/\HubName)};

    \node[minimum size=\NodeScale*\SixScale, inner sep=\innersep] (djrr) at (-0*\HasseSpacingH,6*\HasseSpacingV) {\OldName/\NearName \\ (\MidName/\PathName/\FarName/\HubName)};
    \node[minimum size=\NodeScale*\SixScale, inner sep=\innersep] (drrj) at (2*\HasseSpacingH,6*\HasseSpacingV) {\MidName/\NewName \\ (\PathName/\FarName/\HubName/\rr)};


    
    



    

    % Edges
    \draw (empty) -- (dj);
    \draw (empty) -- (dd);
    \draw (empty) -- (ir);
    \draw (empty) -- (rr);
    \draw (empty) -- (rj);
    
    \draw (dj) -- (djdd);

    \draw (dd) -- (djdd);
    \draw (dd) -- (di);
    \draw (dd) -- (ddir);

    \draw (ir) -- (ddir);
    \draw (ir) -- (irrr);

    \draw (rr) -- (irrr);
    \draw (rr) -- (rrrj);

    \draw (rj) -- (rrrj);

    \draw (djdd) -- (djdi);

    \draw (di) -- (djdi);
    \draw (di) -- (dr);
    \draw (di) -- (diir);

    \draw (ddir) -- (diir);

    \draw (irrr) -- (drrr);
    \draw (irrr) -- (irrj);

    \draw (rrrj) -- (irrj);

    \draw (djdi) -- (djdr);

    \draw (dr) -- (djdr);
    \draw (dr) -- (drir);

    \draw (diir) -- (drir);

    \draw (drir) -- (djir);
    \draw (drir) -- (drrr);
    
    \draw (djdr) -- (djir);

    
    
    \draw (djir) -- (djrr);
    

    \draw (irrj) -- (drrj);
    \draw (drrr) -- (drrj);
    \draw (drrr) -- (djrr);
\end{tikzpicture}
     \end{center}
    \caption{\textbf{Hasse diagram with the 21 transitive closed deletion-invariant causal meta-DAGs with finite ancestral set.}}
    \label{fig:PosetMetaDAG}
\end{figure}

\begin{comment}
\newpage
% \thmNameHasseAppendix
%  \textit{(F\MakeLowercase{amily of causal models})}
\section{Proof of Theorem~\ref{thm:21InvariantCausalModels} \thmNameHasseAppendix}
\label{appendixProof21Regimes}

\textit{For our purpose this is not hard to do by hand, but for more complex things it is worth encode it computationally. \\
A particular handy way to do this is encoding it by matrices . 
for our case we could also encode this on the 8 matrices below***}
\end{comment}
